# Supplementary material for: Conditional Entropy Coding for Efficient Video Compression
Source: arXiv:2008.09180 source file (2020-08-20)
Supplement: Supplementary file 1 [file supp_qual.tex]

\section{Additional Qualitative Results}

\newcommand{\reconc}[3]{
	\begin{overpic}[width=\imw]{#1}
		\put(13,20){ \color{green} \framebox(7, 7){}} 
		\put(55,0){\setlength{\fboxsep}{0pt}\color{green}\fbox{\includegraphics[viewport=252 384 388 518, clip, height=50pt]{#1}}}
		\jcaptiondd{#2}
		\jcaptione{#3}
\end{overpic}}

\newcommand{\trecone}[3]{
	\begin{overpic}[width=\imw]{#1}
		\put(20,32){ \color{green} \framebox(7, 7){}} 
		\put(44,0){\setlength{\fboxsep}{0pt}\color{green}\fbox{\includegraphics[viewport=392 609 529 743, clip, height=60pt]{#1}}}
		\jcaptionf{#2}
		\jcaptiong{#3}
\end{overpic}}
%\newcommand{\jcaptionf}[1]{\put(0,2){\normalsize \colorbox{gray}{\color{white} #1}}}
%\newcommand{\jcaptiong}[1]{\put(0,59){\scriptsize \colorbox{gray}{\color{white} #1}}}
%\newcommand{\trecona}[3]{
%	\begin{overpic}[width=\imw]{#1}
%		\put(20,24){ \color{green} \framebox(8, 8){}} 
%		\put(46,0){\setlength{\fboxsep}{0pt}\color{green}\fbox{\includegraphics[viewport=392 480 548 640, clip, height=86pt]{#1}}}
%		\jcaptionf{#2}
%		\jcaptiong{#3}
%\end{overpic}}
%\newcommand{\jcaptionff}[1]{\put(0,3){\normalsize \colorbox{gray}{\color{white} #1}}}
%\newcommand{\treconb}[3]{
%	\begin{overpic}[width=\imw]{#1}
%		\put(20,24){ \color{green} \framebox(8, 8){}} 
%		\put(46,0){\setlength{\fboxsep}{0pt}\color{green}\fbox{\includegraphics[viewport=392 480 548 640, clip, height=86pt]{#1}}}
%		\jcaptionff{#2}
%		\jcaptiong{#3}
%\end{overpic}}
% teaser figure
\begin{figure*} [!htb]
	\centering
	\def\imw{0.32\textwidth}
	\setlength{\tabcolsep}{1pt}
	\begin{tabular}{ccc}
%		\reconbb{supp_figures/qual_eval/uvg2_recon_cvexp.png}{\textbf{Ours}}{\textbf{[UVG] BPP: 0.025, MS-SSIM: 0.894}} &
%		\reconbb{supp_figures/qual_eval/uvg2_recon_h265.png}{H.265 (veryslow)}{[UVG] BPP: 0.031, MS-SSIM: 0.878} &
%		\reconbb{supp_figures/qual_eval/uvg2_recon_h264.png}{H.264 (veryslow)}{[UVG] BPP: 0.028, MS-SSIM: 0.875}
%		\\ [3pt]
		\reconc{supp_figures/qual_eval/uvg3_recon_cvexp.png}{\textbf{Ours}}{\textbf{[UVG] BPP: 0.076, MS-SSIM: 0.965}} &
		\reconc{supp_figures/qual_eval/uvg3_recon_h265.png}{H.265 (veryslow)}{[UVG] BPP: 0.104, MS-SSIM: 0.959} &
		\reconc{supp_figures/qual_eval/uvg3_recon_h264.png}{H.264 (veryslow)}{[UVG] BPP: 0.088, MS-SSIM: 0.958}
		\\ [3pt]
%		\recond{supp_figures/qual_eval/uvg_recon_cvexp.png}{\textbf{Ours}}{\textbf{[UVG] BPP: 0.076, MS-SSIM: 0.965}} &
%		\recond{supp_figures/qual_eval/uvg_recon_h265.png}{H.265 (veryslow)}{[UVG] BPP: 0.104, MS-SSIM: 0.959} &
%		\recond{supp_figures/qual_eval/uvg_recon_h264.png}{H.264 (veryslow)}{[UVG] BPP: 0.088, MS-SSIM: 0.958}
%		\\ [3pt]
%		\treconc{supp_figures/qual_eval/tor4d_cvexp.png}{\textbf{Ours}}{\textbf{[NorthAmerica] BPP: 0.092, MS-SSIM: 0.975}} &
%		\treconc{supp_figures/qual_eval/tor4d_h265.png}{H.265 (veryslow)}{[NorthAmerica] BPP: 0.114, MS-SSIM: 0.965} &
%		\treconc{supp_figures/qual_eval/tor4d_h264.png}{H.264 (veryslow)}{[NorthAmerica] BPP: 0.105, MS-SSIM: 0.973}
%		\\ [3pt]
%		\trecond{supp_figures/qual_eval/tor4d2_cvexp.png}{\textbf{Ours}}{\textbf{[NorthAmerica] BPP: 0.065, MS-SSIM: 0.983}} &
%		\trecond{supp_figures/qual_eval/tor4d2_h265.png}{H.265 (veryslow)}{[NorthAmerica] BPP: 0.086, MS-SSIM: 0.977} &
%		\trecond{supp_figures/qual_eval/tor4d2_h264.png}{H.264 (veryslow)}{[NorthAmerica] BPP: 0.079, MS-SSIM: 0.977}
%		\\ [3pt]
		\trecone{supp_figures/qual_eval/tor4d3_cvexp.png}{\textbf{Ours}}{\textbf{[NorthAmerica] BPP: 0.047, MS-SSIM: 0.985}} &
		\trecone{supp_figures/qual_eval/tor4d3_h265.png}{H.265 (veryslow)}{[NorthAmerica] BPP: 0.047, MS-SSIM: 0.978} &
		\trecone{supp_figures/qual_eval/tor4d3_h264.png}{H.264 (veryslow)}{[NorthAmerica] BPP: 0.047, MS-SSIM: 0.981}
%		\trecona{figures/qual_eval/tor4d_cvexp.png}{\textbf{Ours}}{\textbf{[NorthAmerica] BPP: 0.087, MS-SSIM: 0.969}} &
%		\treconb{figures/qual_eval/tor4d_h265.png}{H.265 (veryslow)}{[NorthAmerica] BPP: 0.107, MS-SSIM: 0.944} &
%		\treconb{figures/qual_eval/tor4d_h264.png}{H.264 (veryslow)}{[NorthAmerica] BPP: 0.097, MS-SSIM: 0.962}
		\\ [-1pt]
		
	\end{tabular}
	\caption{Additional qualitative demonstration of our approach vs H.265 / H.264 on 12 Hz 1920 $\times$ 1080 UVG video and 10 Hz 1920 $\times$ 1200 NorthAmerica video.}
	\label{fig:qual_eval_supp}
\end{figure*}

%We first provide additional qualitative results in the form of a video, attached as \verb|eccv2020_supp.mp4|. In the video, we highlight our compression framework vs. H.265 \textit{veryslow} on 3 low-framerate video sequences - the first two 12Hz UVG video and the last one 10Hz NorthAmerica video. Our approach outperforms H.265 in these settings in MS-SSIM while achieving a lower bitrate. Qualitatively, we can see that while H.265 tends to introduce motion artifacts within various frames in these low framerate settings, our approach preserves a more even quality of detail within each frame. 

We provide a few more frame comparisons of our approach vs. H.265 \textit{veryslow} and H.264 \textit{veryslow} in Fig. \ref{fig:qual_eval_supp}. We see a similar pattern as demonstrated in the video. Because our reconstructions contain less variance in detail quality, they also contain fewer artifacts compared to H.265 and H.264. We do note, however, that H.265 / H.264 tends to assign more bits to certain high frequency details, such as text, providing slightly sharper outputs than our approach.
